# Supplementary material for: Rare Event Kinetics from Adaptive Bias Enhanced Sampling
Source: arXiv:2208.04942 source file (2022-09-16)
Supplement: Supplementary file 1 [file supp_info.pdf]

# Supplementary Information: Rare Event Kinetics from Adaptive Bias Enhanced Sampling

Dhiman Ray<sup>Δ,†</sup>, Narjes Ansari<sup>Δ,†</sup>, Valerio Rizzi<sup>Δ,†</sup>, Michele Invernizzi,<sup>‡</sup> and Michele Parrinello<sup>\*,†</sup>

<sup>†</sup>*Atomistic Simulations, Italian Institute of Technology, Via Enrico Melen 83, 16152, Genova, Italy*

<sup>‡</sup>*Freie Universität Berlin, Arnimallee 12, 14195, Berlin, Germany*

E-mail: [michele.parrinello@iit.it](mailto:michele.parrinello@iit.it)

<sup>Δ</sup>D.R., N.A. and V.R. contributed equally to the manuscript.

## Supplementary text

### Dimensionality of excluded region $\chi_{\text{exc}}(s)$

For OPES<sub>f</sub> calculations the excluded region  $\chi_{\text{exc}}(s)$  is a function of the collective variables  $s = \{s_1, \dots, s_d\}$ . But depending on the system, the arguments of the  $\chi_{\text{exc}}$  function can be only a subset of  $s$ ,  $s' = \{s'_1, \dots, s'_{d'}\}$ , where  $d' \leq d$  and  $s'_i = s_j$  for some  $i, j$ . One can also decide to use some extra CV  $s_e \neq s_j$  for any  $j$  to demarcate the initial and the transition state more precisely. This is technically possible in the current PLUMED implementation, but it should be noted that the resulting bias potential will no longer be representative of the free energy surface along  $s$ , and Eq. (1) of the main text will no longer hold. As a consequence, the OPES procedure is no longer guaranteed to converge. The bias will effectively be also a function of  $s_e$ , but by construction it will not learn the free energy along  $s_e$ . In practice, one might remain stuck in a basin identified only by  $s_e$ , without the possibility of adapting the bias to exit from it. Thus, extra care should be taken when considering using an excluded region  $\chi_{\text{exc}}$  that is a function of extra CVs. Our suggestion is that if more degrees of freedom are known which can distinguish the initial, final and (or) the transition state, it might be wise to include them in the CV space for biasing to increase the quality of the enhanced sampling simulation and probability reconstruction.

## Identifying $\Delta E$ and $\chi_{\text{exc}}(s)$ from OPES simulation

To choose  $\Delta E$  and  $\chi_{\text{exc}}(s)$  in an optimal manner, the knowledge of the free energy surface is crucial. In the example of chignolin, the  $\sim 100\mu\text{s}$  long unbiased simulation was already available, from which the free energy surface has been constructed prior to the OPES<sub>f</sub> calculations. But this is not the case for any general system, a prior OPES simulation (or other enhanced sampling simulation) may need to be performed to obtain an approximate free energy surface. But the computational cost of such a procedure can be comparable if not larger than the OPES flooding simulation, significantly undermining the efficiency of the overall protocol. Fortunately, the knowledge of the free energy surface only in the initial state basin is sufficient to determine  $\Delta E$  and  $\chi_{\text{exc}}(s)$ . So it is possible to use a harmonic wall to restrict the sampling of the prior OPES simulation in the initial state basin and converging the FES in that region at a minimal computational effort. We attempted to reconstruct the folded state basin of Chignolin for the Deep-LDA and the Deep-TICA coordinate by applying a lowerwall restraint at CV = 0.0, as for neural network based CVs, the two minima are on the two sides of the origin by construction. We show that the FES for the bound state of the chignolin could be estimated within  $\sim 100$  ns of OPES simulation in presence of the wall restraint. The quicker convergence of the FES stems from the fact the transitions between two or more free energy minima is not necessary.

## Construction of Deep-LDA and Deep-TICA CVs for Chignolin

The Deep Linear Discriminant Analysis (Deep-LDA) and the Deep Time-lagged Independent Component Analysis based collective variables for the folding and unfolding of Chignolin were designed following the protocol described in Ref. 1 and 2 respectively. The deep neural networks were trained using the `mlcvs` package (<https://github.com/luigibonati/mlcvs>) and the Pytorch module of Python 3. The PLUMED-Pytorch interface was used to bias the MD simulations along the deep neural network CVs. The details of the training procedure for Deep-LDA and Deep-TICA have been included below.

**Deep-LDA:** For training the Deep-LDA CV, two independent unbiased MD simulation of Chignolin miniprotein have been performed, one starting from the folded state and the another from the unfolded state. The folded state simulation is propagated for  $\sim 22$  ns and the unfolded state simulation is propagated for  $\sim 37$  ns. No transition between the folded and the unfolded state is observed during these simulations. The feature set of 210 interatomic distances suggested by Bonati et al.<sup>2</sup> is used in this study. The value of these features have been recorded at an interval of 1 ps creating a dataset of 22000 samples for the folded state and 37000 for the unfolded state. An 80% of the dataset is used as the training set and the rest is used for validation. A regularization has been applied to the within class scatter matrix ( $\mathbf{S}_W$ ) of the form  $\mathbf{S}_W' = \mathbf{S}_W + \lambda \mathbf{I}$  with  $\lambda = 0.05$ . A neural network with 210-100-60-20-4 architecture and hyperbolic tangent

activation function is used to train the data. The loss function described in SI-1.1 of Ref. 1 is used with an L2 regularization parameter of  $10^{-5}$  and a learning rate of 0.0002.

**Deep-TICA:** The  $\sim 106 \mu\text{s}$  long unbiased trajectory from Ref. 3 is used to train the Deep-TICA CV. The 210 descriptor set identical to the Deep-LDA CV is used as features. The structures have been recorded at an interval of 0.2 ns. A lag time of 5 time steps (i.e. 1 ns) has been used leading to 534736 time-lagged pairs out of which 427788 ( $\sim 80\%$ ) have been used for the training set and the rest 106948 have been used as the validation set. A neural network with architecture 210-50-50-5 and hyperbolic tangent activation function is used. The sum squared loss function described in Eq. 10 of Ref. 2 is used over the first two TICA eigenvectors. Out of the 5 output nodes, only the first node is biased as the CV for the OPES flooding simulations.

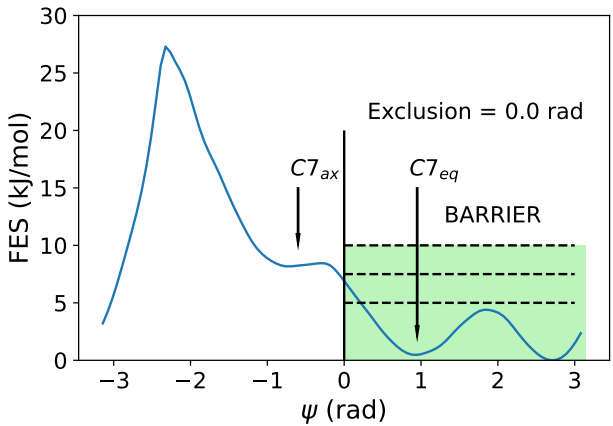

Figure S1: The three different combinations of  $\Delta E$  and  $\chi_{\text{exc}}(s)$  parameters tested for the OPES flooding simulation of the alanine dipeptide biasing the  $\psi$  torsion angle. The free energy surface along the  $\psi$  coordinate is also provided.

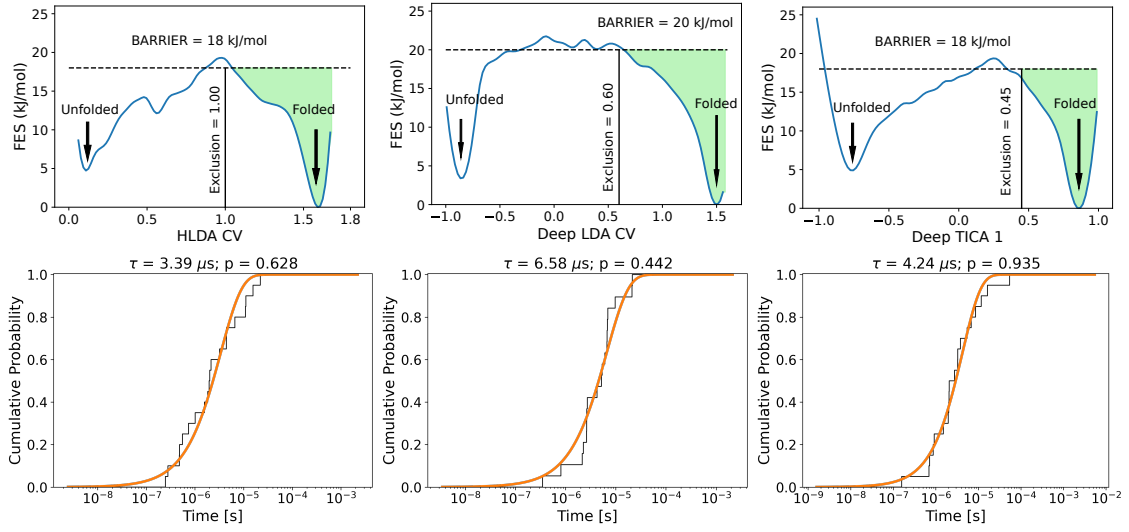

Figure S2: Upper panel: The  $\Delta E$  and  $\chi_{\text{exc}}(s)$  used for the unfolding of Chignolin miniprotein, for the high  $\Delta E$  simulation. In these set up, the  $\Delta E$  is increased as to reach the effective barrier height along the CV. The region flooded with OPES bias is shaded in green. Bottom panel: The quality of Poisson fit of the unfolding timescales.

Table S1: The mean first passage time ( $\tau$ ) of barrier crossing in 2D Wolfe-Quapp Potential with  $\theta = 27^\circ$ , for different values of the  $\Delta E$  and  $s_{\text{exc}}$  parameters. The timescales are reported in the unit of  $10^7$  time steps.

| $\Delta E(k_B T)/s_{\text{exc}}$ | -1    | -0.75 | -0.5  | -0.25 | 0     |
|----------------------------------|-------|-------|-------|-------|-------|
| 4                                | 1.043 | 1.007 | 1.04  | 1.045 | 1.099 |
| 6                                | 1.011 | 1.072 | 1.242 | 1.409 | 1.349 |
| 8                                | 1.216 | 1.684 | 2.324 | 2.517 | 2.738 |
| 10                               | 1.329 | 2.565 | 4.903 | 4.907 | 4.582 |
| 12                               | 1.162 | 2.33  | 5.988 | 8.525 | 7.747 |
| 14                               | 2.169 | 4.215 | 7.448 | 7.32  | 7.251 |
| 16                               | 7.104 | 6.851 | 18.78 | 29.56 | 22.42 |

Table S2: Same as Table S1 but for  $\theta = 54^\circ$

| $\Delta E(k_B T)/s_{exc}$ | -1   | -0.75 | -0.5 | -0.25 | 0    |
|---------------------------|------|-------|------|-------|------|
| 4                         | 0.91 | 1.11  | 1.17 | 1.07  | 1.11 |
| 6                         | 0.9  | 0.96  | 0.96 | 0.89  | 0.91 |
| 8                         | 0.93 | 1.03  | 0.78 | 0.75  | 0.83 |
| 10                        | 0.68 | 0.8   | 1.27 | 1.36  | 1.36 |
| 12                        | 0.95 | 1.36  | 1.68 | 1.65  | 1.63 |
| 14                        | 1.35 | 2.98  | 3.18 | 3.63  | 4.58 |
| 16                        | 2.4  | 4.49  | 7.71 | 11.8  | 17.7 |

Table S3: Same as Table S1 but for  $\theta = 90^\circ$

| $\Delta E(k_B T)/s_{exc}$ | -1.0 | -0.75 | -0.5 | -0.25 | 0.0  |
|---------------------------|------|-------|------|-------|------|
| 4                         | 1.33 | 1.52  | 1.58 | 1.49  | 1.77 |
| 6                         | 1.06 | 0.89  | 0.95 | 0.88  | 1.09 |
| 8                         | 1.37 | 0.76  | 0.68 | 0.71  | 0.63 |
| 10                        | 1.16 | 0.78  | 0.89 | 0.68  | 0.87 |
| 12                        | 1.63 | 0.78  | 0.86 | 0.94  | 0.77 |
| 14                        | 1.05 | 1.36  | 0.89 | 2.06  | 2.03 |
| 16                        | 2.56 | 2.57  | 5.93 | 6.79  | 6.61 |

Table S4: The p-values of the Kolmogorov Smirnov test for the fitting of the  $\tau$  values with the Poisson distribution, for the barrier crossing in 2D Wolfe-Quapp Potential with  $\theta = 27^\circ$ , for different values of the  $\Delta E$  and  $s_{exc}$  parameters.

| $\Delta E(k_B T)/s_{exc}$ | -1    | -0.75 | -0.5  | -0.25 | 0     |
|---------------------------|-------|-------|-------|-------|-------|
| 4                         | 0.971 | 0.899 | 0.818 | 0.968 | 0.953 |
| 6                         | 0.959 | 0.944 | 0.751 | 0.866 | 0.821 |
| 8                         | 0.802 | 0.617 | 0.651 | 0.832 | 0.926 |
| 10                        | 0.976 | 0.473 | 0.496 | 0.158 | 0.142 |
| 12                        | 0.517 | 0.279 | 0.346 | 0.049 | 0.071 |
| 14                        | 0.197 | 0.266 | 0.312 | 0.024 | 0.005 |
| 16                        | 0.058 | 0.015 | 0.002 | 0.223 | 0.03  |

Table S5: Same as Table S4 but for  $\theta = 54^\circ$

| Barrier/Exclusion | -1   | -0.75 | -0.5 | -0.25 | 0    |
|-------------------|------|-------|------|-------|------|
| 4                 | 0.76 | 0.85  | 0.9  | 0.93  | 0.95 |
| 6                 | 0.84 | 0.8   | 0.99 | 0.98  | 0.8  |
| 8                 | 0.7  | 0.95  | 0.77 | 0.57  | 0.8  |
| 10                | 0.44 | 0.46  | 0.95 | 0.68  | 0.72 |
| 12                | 0.11 | 0.57  | 0.13 | 0.57  | 0.08 |
| 14                | 0.08 | 0.07  | 0.02 | 0.11  | 0.03 |
| 16                | 0.01 | 0.02  | 0.03 | 0.02  | 0.07 |

Table S6: Same as Table S4 but for  $\theta = 90^\circ$

| $\Delta E(k_B T)/s_{exc}$ | -1.0 | -0.75 | -0.5  | -0.25 | 0.0   |
|---------------------------|------|-------|-------|-------|-------|
| 4                         | 0.55 | 0.91  | 0.89  | 0.95  | 0.94  |
| 6                         | 0.96 | 0.94  | 0.87  | 0.95  | 0.99  |
| 8                         | 0.79 | 0.94  | 0.78  | 0.54  | 0.44  |
| 10                        | 0.71 | 0.73  | 0.73  | 0.88  | 0.50  |
| 12                        | 0.85 | 0.10  | 0.003 | 0.015 | 0.004 |
| 14                        | 0.05 | 0.16  | 0.008 | 0.033 | 0.021 |
| 16                        | 0.01 | 0.02  | 0.10  | 0.02  | 0.03  |

Table S7: The  $\tau$  of conformational transition in the alanine dipeptide with bias applied along the  $\psi$  torsion angle, and for different values of the  $\Delta E$  and  $s_{exc}$  parameters. The timescales are reported in  $\mu s$ . The unbiased estimate is  $\tau = 1.28 \mu s$

| $\Delta E$ (kJ/mol)/ $s_{exc}$ (rad) | -0.7 | -0.6 | -0.5 | -0.4 | -0.3 | -0.2 | -0.1 |
|--------------------------------------|------|------|------|------|------|------|------|
| 15                                   | 0.69 | 0.96 | 1.07 | 0.91 | 0.89 | 1.29 | 1.04 |
| 20                                   | 1.11 | 0.82 | 1.02 | 1.11 | 1.13 | 1.17 | 1.21 |
| 25                                   | 1.12 | 0.96 | 0.9  | 0.86 | 0.71 | 0.74 | 0.98 |
| 30                                   | 1.43 | 1.71 | 1.13 | 2    | 1.59 | 1.38 | 1.27 |
| 35                                   | 1.36 | 2.15 | 3.76 | 8.23 | 2.39 | 1.36 | 4.89 |
| 40                                   | 16.9 | 26.1 | 18.7 | 23.5 | 25   | 23.5 | 16.5 |

Table S8: Same as Table S7 but for the p-values of the Kolmogorov Smirnov test for the Poisson fitting of the kinetic results.

| $\Delta E$ (kJ/mol)/ $s_{exc}$ (rad) | -0.7  | -0.6 | -0.5 | -0.4  | -0.3 | -0.2 | -0.1 |
|--------------------------------------|-------|------|------|-------|------|------|------|
| 15                                   | 0.6   | 0.35 | 0.67 | 0.98  | 0.53 | 0.59 | 0.3  |
| 20                                   | 0.39  | 0.69 | 0.9  | 0.996 | 0.74 | 0.25 | 0.84 |
| 25                                   | 0.997 | 0.94 | 0.42 | 0.47  | 0.72 | 0.8  | 0.83 |
| 30                                   | 0.58  | 0.76 | 0.82 | 0.6   | 0.64 | 0.89 | 0.33 |
| 35                                   | 0.64  | 0.81 | 0.46 | 0.94  | 0.96 | 0.18 | 0.28 |
| 40                                   | 0.7   | 0.78 | 0.59 | 0.91  | 0.61 | 0.62 | 0.11 |

Table S9: Same as Table S7 but for the acceleration factor ( $\tau/\tau_f$ )

| $\Delta E$ (kJ/mol)/ $s_{exc}$ (rad) | -0.7    | -0.6    | -0.5   | -0.4    | -0.3    | -0.2   | -0.1    |
|--------------------------------------|---------|---------|--------|---------|---------|--------|---------|
| 15                                   | 430     | 447     | 460    | 465     | 467     | 473    | 473     |
| 20                                   | 2652    | 2690    | 2754   | 2856    | 2861    | 2938   | 2881    |
| 25                                   | 11659   | 12030   | 13497  | 11943   | 12012   | 12925  | 12566   |
| 30                                   | 44569   | 46612   | 47904  | 52596   | 53123   | 50880  | 53593   |
| 35                                   | 45799   | 54858   | 235425 | 288450  | 59531   | 52015  | 236030  |
| 40                                   | 1001981 | 1046662 | 895861 | 1236462 | 1233448 | 910016 | 1293761 |

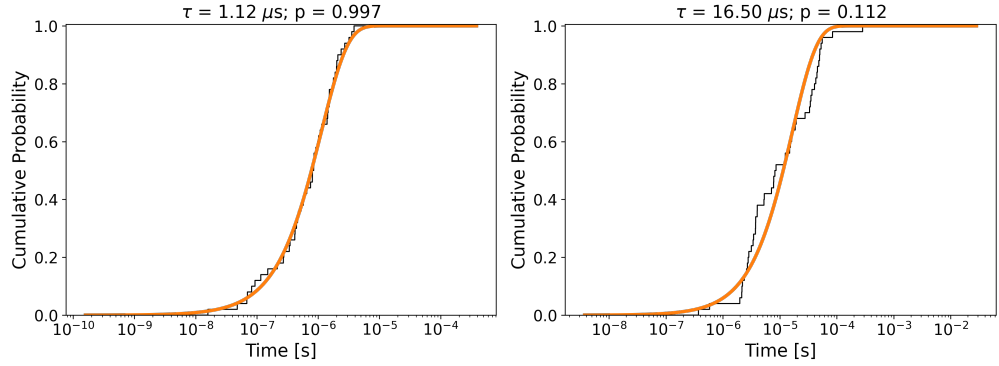

Figure S3: The quality of fit of the reweighted transition times in alanine dipptide with the Poisson distribution. The left subplot indicates an ideal scenario i.e. low  $\Delta E$  (25 kJ/mol) and larger excluded region ( $s_{exc} = -0.7$  rad). The predicted  $\tau$  is closer to the unbiased estimate, and the degree of fit is good ( $p \approx 1$ ). The right panel shows a pathological situation where  $\Delta E$  (40 kJ/mol) is higher than the activation barrier and only a limited region is excluded from bias deposition ( $s_{exc} = -0.1$  rad). The  $\tau$  is overestimated by more than one order of magnitude and the degree of fit is poor ( $p \ll 1$ ).

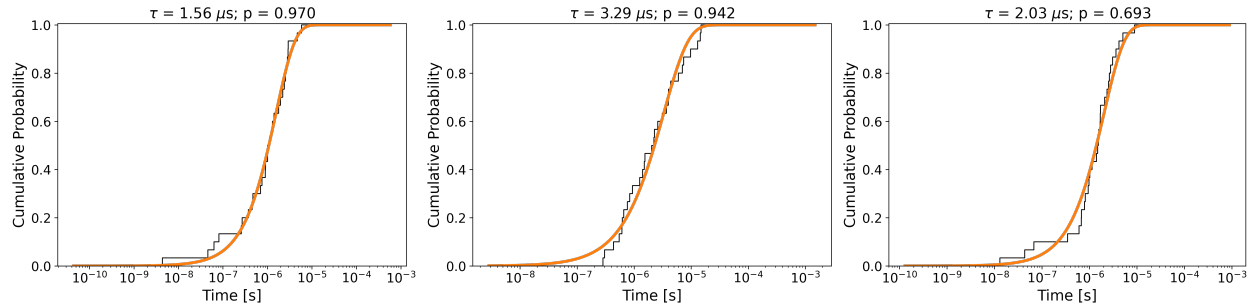

Figure S4: The Poisson fit of the reweighted transition times in alanine dipptide when the  $\psi$  CV is biased during OPES flooding. The subplots are for  $\Delta E = 5, 7.5$ , and 10 kJ/mol barrier parameter from left to right.

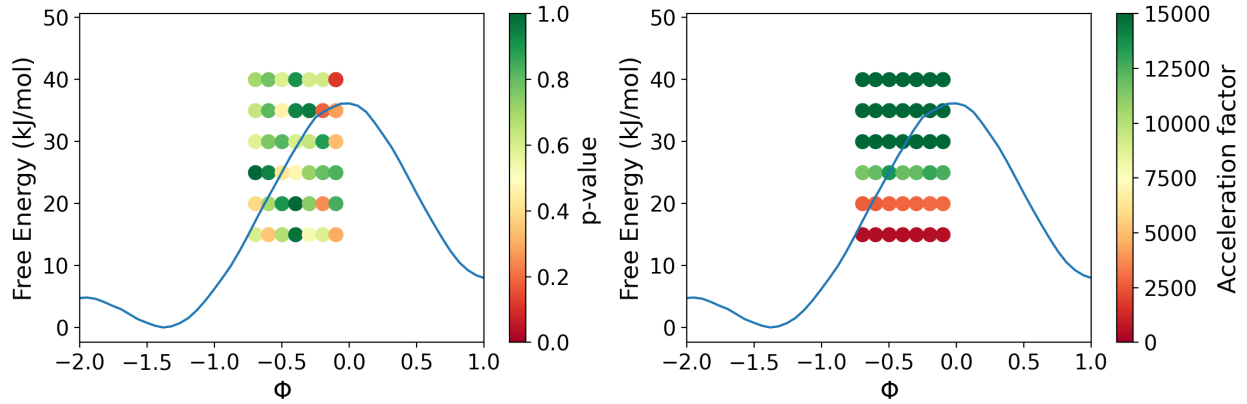

Figure S5: The change of p-value and acceleration factor for different combinations of  $\Delta E$  and  $s_{exc}$  parameters for alanine dipeptide with bias applied along  $\phi$  CV. For a detailed description, see Fig. 3 and Fig. 4 in the main text.

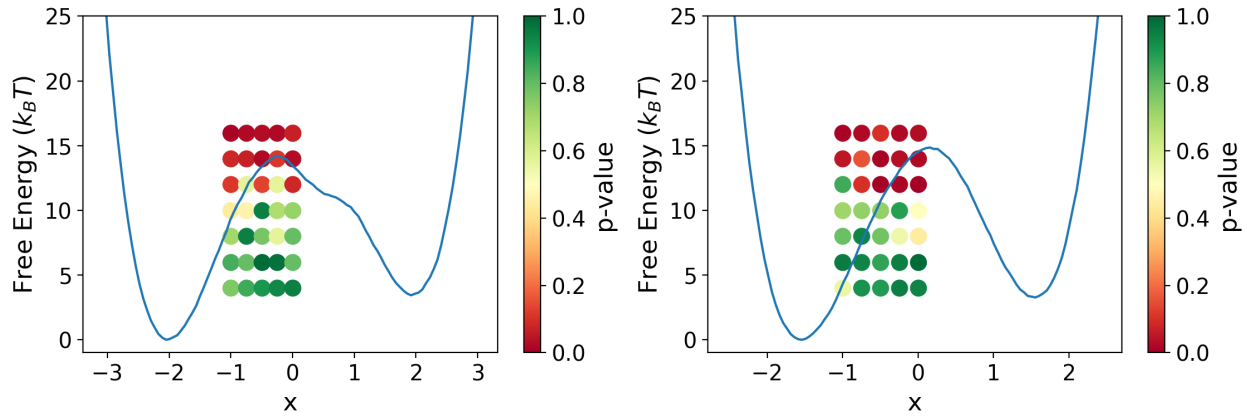

Figure S6: The change of p-value for the Kolmogorov Smirnov test of the kinetics for OPES flooding simulation for the 2D Wolfe-Quapp potential, with different combinations of  $\Delta E$  and  $s_{exc}$ . The left figure is for  $\theta = 54^\circ$  and the right plot is for  $\theta = 90^\circ$

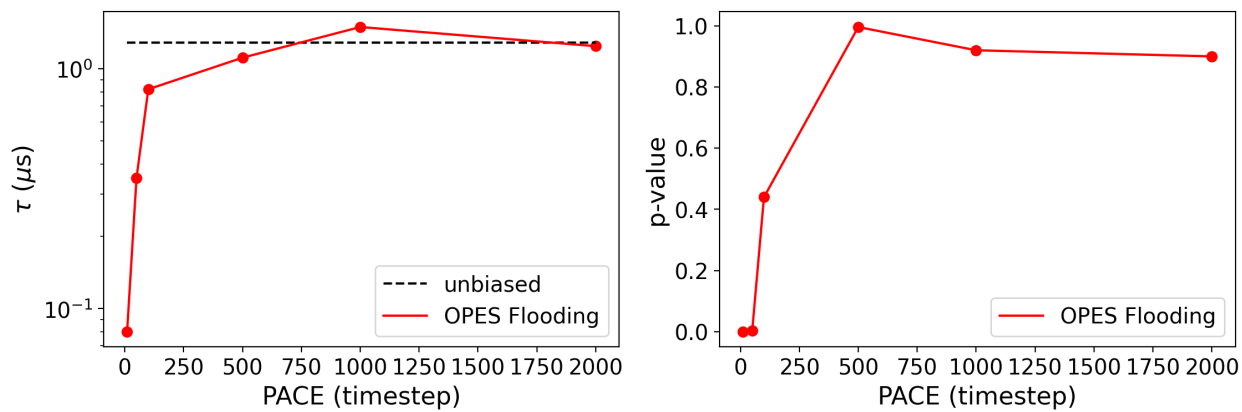

Figure S7: The dependence of the quality of the kinetic results obtained from OPES flooding on the PACE parameter (i.e. the frequency of deposition of Gaussian Kernels). The results shown here are for the alanine dipeptide system with  $\phi$  torsion angle as CV.

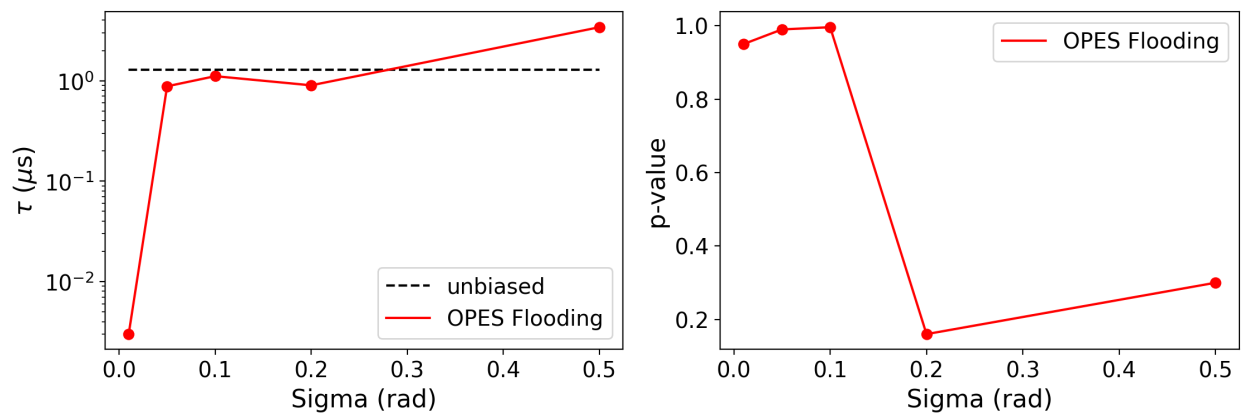

Figure S8: The dependence of the quality of the kinetic results obtained from OPES flooding on the SIGMA parameter (i.e. the initial width of the deposited Gaussian Kernels). The results shown here are for the alanine dipeptide system with  $\phi$  torsion angle as CV. The default SIGMA parameter estimated by the OPES protocol is  $\sim 0.47$  rad.

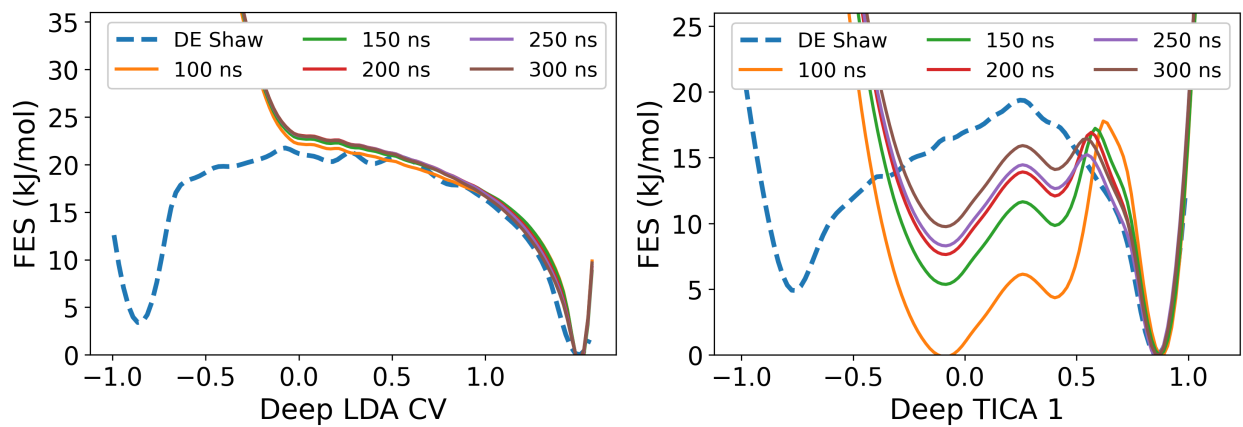

Figure S9: Free energy surface of the folded state of chignolin miniprotein constructed from OPES simulation with harmonic wall restraint along the Deep-LDA CV (left) and the Deep-TICA CV (right). The free energy surface obtained from the long unbiased simulation from Ref. 3 by DE Shaw research is shown as a reference.

Table S10: Results of unfolding kinetics of chignolin from OPES flooding simulation using the higher  $\Delta E$  parameter set.

| Method/CV | $\tau$ ( $\mu$ s) | p    | $\mu$ | $\sigma$ | Acceleration factor |
|-----------|-------------------|------|-------|----------|---------------------|
| Unbiased  | 2.2               | -    | -     | -        | -                   |
| HLDA      | 3.39              | 0.63 | 4.58  | 5.77     | 160                 |
| Deep-LDA  | 6.58              | 0.44 | 6.12  | 5.69     | 597                 |
| Deep-TICA | 4.24              | 0.93 | 6.47  | 11.7     | 360                 |

Table S11: Results of folding kinetics of chignolin from OPES flooding simulation using lower  $\Delta E$  parameter set.

| Method/CV | $\tau$ ( $\mu$ s) | p-value | $\mu$ | $\sigma$ | Acceleration factor | $\Delta E$ (kJ/mol) |
|-----------|-------------------|---------|-------|----------|---------------------|---------------------|
| Unbiased  | 0.60              | -       | -     | -        | -                   | -                   |
| HLDA      | 1.61              | 0.59    | 1.38  | 1.04     | 10                  | 7                   |
| Deep-LDA  | 1.90              | 0.94    | 1.90  | 1.84     | 32                  | 8                   |
| Deep-TICA | 0.85              | 0.99    | 0.78  | 0.64     | 17                  | 7                   |

Table S12: Results of folding kinetics of chignolin from OPES flooding simulation using the higher  $\Delta E$  parameter set.

| Method/CV | $\tau$ ( $\mu$ s) | p-value | $\mu$ | $\sigma$ | Acceleration factor | $\Delta E$ (kJ/mol) |
|-----------|-------------------|---------|-------|----------|---------------------|---------------------|
| Unbiased  | 0.60              | -       | -     | -        | -                   | -                   |
| HLDA      | 6.46              | 0.91    | 7.08  | 7.50     | 86                  | 13                  |
| Deep-LDA  | 3.36              | 0.72    | 5.50  | 7.94     | 374                 | 17                  |
| Deep-TICA | 2.16              | 0.21    | 2.14  | 2.19     | 121                 | 13                  |

## References

- (1) Bonati, L.; Rizzi, V.; Parrinello, M. Data-Driven Collective Variables for Enhanced Sampling. *The Journal of Physical Chemistry Letters* **2020**, *11*, 2998–3004.
- (2) Bonati, L.; Piccini, G.; Parrinello, M. Deep learning the slow modes for rare events sampling. *Proceedings of the National Academy of Sciences* **2021**, *118*.
- (3) Lindorff-Larsen, K.; Piana, S.; Dror, R. O.; Shaw, D. E. How Fast-Folding Proteins Fold. *Science* **2011**, *334*, 517–520.
